# Supplementary material for: Atiyah-Hirzebruch spectral sequence for topological insulators and superconductors: $E_2$ pages for 1651 magnetic space groups
Source: arXiv:2304.01827 ancillary file (2026-05-02)
Supplement: Supplementary file 1 [file SM.pdf]

# Supplimental Material for "Atiyah-Hirzebruch Spectral Sequence for topological insulators and superconductors: $E_2$ pages for 1651 magnetic space groups"

Ken Shiozaki[1] and Seishiro Ono[2,*]

[1]*Center for Gravitational Physics and Quantum Information, Yukawa Institute for Theoretical Physics, Kyoto University, Kyoto 606-8502, Japan*

[2]*Department of Applied Physics, University of Tokyo, Tokyo 113-8656, Japan*

(Dated: April 4, 2023)

Supplemental Material includes two txt files:

- `ExtensionList.txt`

- `E2.txt`

Here, we explain the structure and how to read the data for each.

Each line in `ExtensionList.txt` has the following structure:

$$\{A, B, \{E_0, E_1, E_2, ...\}\}.$$

Here, $A, B, E_0, E_1, E_2, ...$ are sets of non-negative integers, representing a single $\mathbb{Z}$-module for each. 0 represents $\mathbb{Z}$, and a non-zero integer $n$ represents $\mathbb{Z}_n$. For example,

$$\{\{4\}, \{0, 2\}, \{\{0, 2\}, \{0, 4\}, \{0, 8\}, \{0, 2, 2\}, \{0, 4, 2\}\}\}$$

indicates that for the $\mathbb{Z}$-module $A = \mathbb{Z}_4$, there are five possible $\mathbb{Z}$-modules resulting from the extension by $B = \mathbb{Z} \oplus \mathbb{Z}_2$: $\mathbb{Z} \oplus \mathbb{Z}_2, \mathbb{Z} \oplus \mathbb{Z}_4, \mathbb{Z} \oplus \mathbb{Z}_8, \mathbb{Z} \oplus \mathbb{Z}_2^{\oplus 2}, \mathbb{Z} \oplus \mathbb{Z}_4 \oplus \mathbb{Z}_2$.

Each line in `E2.txt` consists of 12 elements, and the meaning and description of each are summarized in the table

* Present address: Interdisciplinary Theoretical and Mathematical Sciences Program (iTHEMS), RIKEN, Wako 351-0198, Japan

below.

| | | |
|---|---|---|
| 1 | Spatial dimension | Takes a value of 1, 2, or 3. |
| 2 | Presence or absence of lattice translational symmetry | Takes one of the values "MSG", "MLG", "MRG", or "MPG". "MSG", "MLG", and "MRG" are symmetry groups with lattice translational symmetry and represent magnetic space groups, magnetic layer groups, and magnetic rod groups, respectively. "MPG" is a symmetry group without lattice translational symmetry and represents a magnetic point group. |
| 3 | Insulator/Superconductor | Takes one of the values "TI" or "SC", representing insulators and superconductors, respectively. |
| 4 | Factor system of electrons | Takes a value of either "Spinless" or "Spinful", representing spinless electron systems and spinful electron systems, respectively. |
| 5 | Number of symmetry groups | For "MSG", it represents the BNS number, e.g., "69.524". For "MLG" and "MRG", it represents the OG number in [1], e.g., "31.4.191". For "MPG", there is no number, and the value is "n/a". |
| 6 | Symbol of the symmetry group | For "MSG", "MLG", and "MRG", it takes the BNS symbol, e.g., "P_c42_12". The BNS symbols for "MLG" and "MRG" are taken from [1]. For "MPG", the symbol of magnetic point group symmetry is used. |
| 7 | Type of particle-hole symmetry | For "SC", it takes a value of either "D" or "C", representing whether the square of the particle-hole operation is 1 or -1, corresponding to Altland-Zirnbauer symmetry class D and C, respectively. For "TI", it does not apply, and the value is "n/a". |
| 8 | Character table of pairing symmetry | The first row consists of $O(3)$ rotation matrices of the point group, and the second row consists of the corresponding characters of a one-dimensional representation of pairing symmetry. For "TI", it does not apply, and the value is "n/a". |
| 9 | Symbol of pairing symmetry | Takes a value of the symbol of one-dimensional representation, e.g., "A_1g". For "TI", it does not apply, and the value is "n/a". |
| 10 | $E_2$-page of momentum-space AHSS | An $8 \times (\text{spatial dimension} + 1)$ dimensional matrix, where the row and column numbers, counted from 0, represent the $n$ and $p$ in the $E_2$-page $E_2^{p,-n}$, respectively. Matrix elements consist of non-negative integer sets specifying $\mathbb{Z}$-modules, where 0 represents $\mathbb{Z}$ and a natural number represents $\mathbb{Z}_n$. |
| 11 | $E^2$-page of real-space AHSS | An $8 \times (\text{spatial dimension} + 1)$ dimensional matrix, where the row and column numbers, counted from 0, represent the $n$ and $p$ in the $E^2$-page $E^2_{p,-n}$, respectively. Matrix elements consist of non-negative integer sets specifying $\mathbb{Z}$-modules, where 0 represents $\mathbb{Z}$ and a natural number represents $\mathbb{Z}_n$. |
| 12 | Set of candidate $K$-groups | An array with 8 elements, representing the set of $\mathbb{Z}$-modules that can be candidate $K$-groups for ${}^{\phi}K_G^{(z,c)+n}(X_{\mathrm{k}}) \cong {}^{\phi}K^{\mathcal{G}}_{(z^{\mathrm{int}},c)-n}(X_{\mathrm{r}})$ with $n = 0, 1, \ldots, 7$. (Here, $X_{\mathrm{k}}$ refers to momentum space, and $X_{\mathrm{r}}$ refers to real space.) $\mathbb{Z}$-modules are specified by non-negative integer sets, where 0 represents $\mathbb{Z}$ and a natural number represents $\mathbb{Z}_n$. |

[1] D. B. Litvin, Magnetic group tables, International Union of Crystallography (2013).
